# Supplementary material for: Maximum pseudo-likelihood estimation based on estimated residuals in copula semiparametric models
Source: arXiv:1903.04221 ancillary file (2019-03-11)
Supplement: Supplementary file 1 [file suplement.pdf]

Supplementary material to the article:

# Maximum pseudolikelihood estimation based on estimated residuals in copula semiparametric models

Marek Omelka, Šárka Hudecová, Natalie Neumeyer

## 1 Supplement to simulation study

The following model was considered in a Monte Carlo study

$$\begin{aligned} Y_{1i} &= \theta_{10} + \theta_{11} X_i + \varepsilon_{1i}, \\ Y_{2i} &= \theta_{20} + \theta_{21} X_i + \varepsilon_{2i}. \end{aligned} \tag{1}$$

In the main article, we discuss properties of the estimators based on residuals for Clayton, Frank, and Gaussian copula. Here we provide results for model (1) with $C$ being Gumbel or Student copula with 5 degrees of freedom. First of all, note that for the Gumbel copula in Table 1, the marginal distribution function $F_{2\varepsilon}$ is not exponential in the case N+E, but corresponds to the distribution function of $-U$, where $U$ is exponential with mean 1. Hence, the corresponding density $f_{2\varepsilon}$ has a jump at the right end of its support. For this choice of marginals, the pseudo-maximum likelihood estimator $\widehat{\alpha}^{(pl)}$ is visibly biased even for $\tau = 0.5$. For $\tau = 0.75$ the standard deviation is noticeably larger as well. In this case, the modified estimator $\widehat{\alpha}^{(pl*)}$ helps to reduce both quantities. If the marginal $F_{2\varepsilon}$ is uniform, then the performance of $\widehat{\alpha}^{(pl)}$ seems to be good for $\tau = 0.5$, but for $\tau = 0.75$ there is a visible bias. The modified estimator successfully reduces this bias, and for $n = 10\,000$ this estimator performs similarly as the estimator $\widehat{\alpha}^{(ik)}$ based on Kendall's tau. For $t$ marginals, the behavior is analogous as described for the Clayton copula.

Table 2 provides results for model (1) for Student copula $C$. The performance of the estimators resembles o the Gaussian copula, discussed in the main article.

To illustrate the results for $d = 3$, the following model was considered

$$\begin{aligned} Y_{1i} &= \theta_{10} + \theta_{11} X_{1i} + \theta_{12} X_{2i} + \varepsilon_{1i}, \\ Y_{2i} &= \theta_{20} + \theta_{21} X_{1i} + \theta_{22} X_{2i} + \varepsilon_{1i}, \\ Y_{3i} &= \theta_{30} + \theta_{31} X_{1i} + \theta_{32} X_{2i} + \varepsilon_{1i}, \end{aligned} \tag{2}$$

$i = 1, \ldots, n$. The joint distribution of $(\varepsilon_{1i}, \varepsilon_{2i}, \varepsilon_{3i})^\top$ is $C(F_{1\varepsilon}(y_1), F_{2\varepsilon}(y_2), F_{3\varepsilon}(y_3))$, where $C$ is copula being one of Clayton, Frank, Gumbel, and normal, the marginals $F_{1\varepsilon}$ and $F_{2\varepsilon}$ are standard normal, while the marginal distribution function $F_{3\varepsilon}$ is either exponential with mean 1 or uniform on $[-1, 1]$. The parameters of the copulas are chosen such that they correspond to Kendall's tau $\tau = 0.5$ and $\tau = 0.75$. For normal and Student copula, the exchangeable correlation structure is considered. The regressors $(X_{1i}, X_{2i})^\top$ are generated from bivariate normal distribution with zero means, unit variances, and correlation $\rho$ being

0.5. The bias, SD, and RMSE of the five estimators listed above (recomputed again on the Kendall's tau scale) are calculated from 1 000 random samples of sample sizes $n = 100,\ 1\,000,\ 10\,000$, and are multiplied by 100. The presented results correspond to the model parameters $(\theta_{10}, \theta_{11}, \theta_{12})^\top = (1, 1, 1)^\top$, $(\theta_{20}, \theta_{21}, \theta_{22})^\top = (1, -1/3, 1/3)^\top$, and $(\theta_{30}, \theta_{31}, \theta_{32})^\top = (0, -1/2, -1/2)^\top$.

Based on the results in Tables 3, 4, 5, 6, conclusions analogous to those in previous section can be made regarding the behavior of the estimators. Similarly as for model (1), results for $F_{3\varepsilon}$ corresponding to $-U$ with $U$ being exponential with mean 1 are presented for the Gumbel copula for the N+N+E situation.

| $\tau$ | Marginals | estim | $n = 100$ | | | $n = 1\,000$ | | | $n = 10\,000$ | | |
|---|---|---|---|---|---|---|---|---|---|---|---|
| | | | bias | SD | RMSE | bias | SD | RMSE | bias | SD | RMSE |
| 0.50 | inov | $\widetilde{\alpha}^{(ik)}$ | 0.03 | 5.29 | 5.29 | −0.03 | 1.66 | 1.66 | 0.00 | 0.51 | 0.51 |
| | | $\widetilde{\alpha}^{(pl)}$ | 0.85 | 5.03 | 5.10 | 0.08 | 1.61 | 1.61 | 0.01 | 0.50 | 0.50 |
| | N+E | $\widehat{\alpha}^{(ik)}$ | −0.86 | 5.30 | 5.37 | −0.21 | 1.67 | 1.69 | −0.02 | 0.51 | 0.51 |
| | | $\widehat{\alpha}^{(pl)}$ | −1.56 | 5.18 | 5.41 | −0.98 | 1.76 | 2.01 | −0.38 | 0.57 | 0.68 |
| | | $\widehat{\alpha}^{(pl*)}$ | −0.10 | 5.25 | 5.25 | −0.37 | 1.71 | 1.75 | −0.15 | 0.53 | 0.55 |
| | N+U | $\widehat{\alpha}^{(ik)}$ | −0.10 | 5.34 | 5.34 | −0.06 | 1.66 | 1.66 | 0.00 | 0.51 | 0.51 |
| | | $\widehat{\alpha}^{(pl)}$ | 0.24 | 5.05 | 5.05 | −0.20 | 1.60 | 1.61 | −0.10 | 0.50 | 0.51 |
| | | $\widehat{\alpha}^{(pl*)}$ | 1.06 | 5.27 | 5.37 | 0.14 | 1.64 | 1.64 | 0.03 | 0.50 | 0.50 |
| | t | $\widehat{\alpha}^{(ik)}$ | 0.04 | 5.33 | 5.33 | −0.03 | 1.67 | 1.67 | 0.00 | 0.51 | 0.51 |
| | | $\widehat{\alpha}^{(pl)}$ | 0.79 | 5.10 | 5.16 | 0.07 | 1.61 | 1.61 | 0.01 | 0.49 | 0.49 |
| | | $\widehat{\alpha}^{(pl*)}$ | 1.24 | 5.27 | 5.41 | 0.20 | 1.65 | 1.66 | 0.06 | 0.50 | 0.50 |
| 0.75 | inov | $\widetilde{\alpha}^{(ik)}$ | −0.01 | 3.14 | 3.14 | 0.02 | 0.96 | 0.96 | 0.01 | 0.30 | 0.30 |
| | | $\widetilde{\alpha}^{(pl)}$ | −0.22 | 2.91 | 2.91 | −0.03 | 0.90 | 0.90 | 0.00 | 0.28 | 0.28 |
| | N+E | $\widehat{\alpha}^{(ik)}$ | −1.48 | 3.31 | 3.63 | −0.31 | 1.00 | 1.05 | −0.04 | 0.31 | 0.31 |
| | | $\widehat{\alpha}^{(pl)}$ | −4.10 | 3.74 | 5.54 | −1.96 | 1.59 | 2.53 | −0.72 | 0.58 | 0.92 |
| | | $\widehat{\alpha}^{(pl*)}$ | −2.63 | 3.47 | 4.35 | −1.21 | 1.36 | 1.82 | −0.44 | 0.48 | 0.65 |
| | N+U | $\widehat{\alpha}^{(ik)}$ | −0.25 | 3.14 | 3.15 | −0.03 | 0.96 | 0.96 | 0.00 | 0.30 | 0.30 |
| | | $\widehat{\alpha}^{(pl)}$ | −1.18 | 2.94 | 3.17 | −0.57 | 0.95 | 1.11 | −0.21 | 0.31 | 0.37 |
| | | $\widehat{\alpha}^{(pl*)}$ | −0.46 | 2.96 | 3.00 | −0.18 | 0.92 | 0.94 | −0.06 | 0.29 | 0.30 |
| | t | $\widehat{\alpha}^{(ik)}$ | −0.08 | 3.17 | 3.17 | 0.01 | 0.96 | 0.96 | 0.01 | 0.30 | 0.30 |
| | | $\widehat{\alpha}^{(pl)}$ | −0.33 | 2.91 | 2.93 | −0.04 | 0.90 | 0.90 | 0.00 | 0.28 | 0.28 |
| | | $\widehat{\alpha}^{(pl*)}$ | −0.18 | 2.97 | 2.97 | 0.02 | 0.91 | 0.91 | 0.02 | 0.28 | 0.28 |

Table 1: Model (1) with Gumbel copula, quantities multiplied by 100

| $\tau$ | Marginals | estim | $n = 100$ | | | $n = 1\,000$ | | | $n = 10\,000$ | | |
|---|---|---|---|---|---|---|---|---|---|---|---|
| | | | bias | SD | RMSE | bias | SD | RMSE | bias | SD | RMSE |
| 0.50 | inov | $\widetilde{\alpha}^{(ik)}$ | −0.07 | 5.56 | 5.56 | 0.00 | 1.75 | 1.74 | 0.02 | 0.52 | 0.52 |
| | | $\widetilde{\alpha}^{(pl)}$ | 0.83 | 5.34 | 5.40 | 0.12 | 1.68 | 1.68 | 0.04 | 0.51 | 0.51 |
| | N+E | $\widehat{\alpha}^{(ik)}$ | −0.62 | 5.58 | 5.62 | −0.12 | 1.75 | 1.75 | 0.01 | 0.52 | 0.52 |
| | | $\widehat{\alpha}^{(pl)}$ | −0.30 | 5.30 | 5.30 | −0.32 | 1.70 | 1.72 | −0.10 | 0.52 | 0.53 |
| | | $\widehat{\alpha}^{(pl*)}$ | 0.61 | 5.54 | 5.57 | 0.06 | 1.72 | 1.72 | 0.04 | 0.51 | 0.51 |
| | N+U | $\widehat{\alpha}^{(ik)}$ | −0.17 | 5.58 | 5.58 | −0.02 | 1.74 | 1.74 | 0.02 | 0.52 | 0.52 |
| | | $\widehat{\alpha}^{(pl)}$ | 0.42 | 5.28 | 5.29 | −0.07 | 1.67 | 1.67 | −0.03 | 0.51 | 0.51 |
| | | $\widehat{\alpha}^{(pl*)}$ | 1.12 | 5.55 | 5.66 | 0.25 | 1.71 | 1.73 | 0.09 | 0.51 | 0.52 |
| | t | $\widehat{\alpha}^{(ik)}$ | −0.02 | 5.61 | 5.61 | 0.00 | 1.75 | 1.74 | 0.02 | 0.52 | 0.52 |
| | | $\widehat{\alpha}^{(pl)}$ | 0.84 | 5.38 | 5.45 | 0.11 | 1.68 | 1.68 | 0.04 | 0.51 | 0.51 |
| | | $\widehat{\alpha}^{(pl*)}$ | 1.27 | 5.51 | 5.65 | 0.30 | 1.71 | 1.74 | 0.10 | 0.51 | 0.52 |
| 0.75 | inov | $\widetilde{\alpha}^{(ik)}$ | −0.05 | 3.20 | 3.20 | −0.03 | 0.96 | 0.96 | −0.01 | 0.30 | 0.30 |
| | | $\widetilde{\alpha}^{(pl)}$ | −0.20 | 2.94 | 2.95 | −0.03 | 0.87 | 0.87 | −0.01 | 0.28 | 0.28 |
| | N+E | $\widehat{\alpha}^{(ik)}$ | −1.26 | 3.22 | 3.46 | −0.27 | 0.98 | 1.02 | −0.05 | 0.30 | 0.31 |
| | | $\widehat{\alpha}^{(pl)}$ | −2.35 | 3.14 | 3.93 | −0.90 | 1.08 | 1.41 | −0.30 | 0.35 | 0.46 |
| | | $\widehat{\alpha}^{(pl*)}$ | −1.49 | 3.06 | 3.40 | −0.53 | 1.02 | 1.15 | −0.18 | 0.33 | 0.37 |
| | N+U | $\widehat{\alpha}^{(ik)}$ | −0.30 | 3.20 | 3.21 | −0.07 | 0.96 | 0.97 | −0.02 | 0.30 | 0.30 |
| | | $\widehat{\alpha}^{(pl)}$ | −0.97 | 2.90 | 3.06 | −0.41 | 0.93 | 1.02 | −0.16 | 0.30 | 0.34 |
| | | $\widehat{\alpha}^{(pl*)}$ | −0.32 | 2.93 | 2.95 | −0.11 | 0.90 | 0.91 | −0.05 | 0.29 | 0.29 |
| | t | $\widehat{\alpha}^{(ik)}$ | −0.09 | 3.22 | 3.22 | −0.03 | 0.96 | 0.96 | −0.01 | 0.30 | 0.30 |
| | | $\widehat{\alpha}^{(pl)}$ | −0.24 | 2.95 | 2.96 | −0.03 | 0.87 | 0.87 | −0.02 | 0.28 | 0.28 |
| | | $\widehat{\alpha}^{(pl*)}$ | −0.06 | 2.94 | 2.94 | 0.03 | 0.89 | 0.89 | 0.01 | 0.28 | 0.28 |

Table 2: Model (1) with Student copula, quantities multiplied by 100

| $\tau$ | Marginals | estim | $n = 100$ | | | $n = 1\,000$ | | | $n = 10\,000$ | | |
|---|---|---|---|---|---|---|---|---|---|---|---|
| | | | bias | SD | RMSE | bias | SD | RMSE | bias | SD | RMSE |
| 0.50 | inov | $\widetilde{\alpha}^{(ik)}$ | 0.20 | 4.60 | 4.60 | 0.07 | 1.38 | 1.38 | -0.01 | 0.43 | 0.43 |
| | | $\widetilde{\alpha}^{(pl)}$ | 0.02 | 4.15 | 4.14 | -0.01 | 1.29 | 1.29 | -0.02 | 0.40 | 0.40 |
| | N+N+E | $\widehat{\alpha}^{(ik)}$ | -1.24 | 4.61 | 4.77 | -0.24 | 1.38 | 1.40 | -0.06 | 0.43 | 0.43 |
| | | $\widehat{\alpha}^{(pl)}$ | -5.05 | 4.27 | 6.61 | -2.58 | 1.63 | 3.05 | -1.03 | 0.64 | 1.21 |
| | | $\widehat{\alpha}^{(pl*)}$ | -3.08 | 4.21 | 5.21 | -1.61 | 1.50 | 2.20 | -0.66 | 0.57 | 0.87 |
| | N+N+U | $\widehat{\alpha}^{(ik)}$ | 0.02 | 4.61 | 4.61 | 0.03 | 1.38 | 1.38 | -0.02 | 0.43 | 0.43 |
| | | $\widehat{\alpha}^{(pl)}$ | -1.58 | 4.05 | 4.34 | -0.74 | 1.25 | 1.45 | -0.31 | 0.42 | 0.52 |
| | | $\widehat{\alpha}^{(pl*)}$ | -0.59 | 4.10 | 4.14 | -0.27 | 1.27 | 1.30 | -0.12 | 0.40 | 0.42 |
| 0.75 | inov | $\widetilde{\alpha}^{(ik)}$ | 0.13 | 2.82 | 2.82 | 0.08 | 0.86 | 0.86 | -0.01 | 0.28 | 0.28 |
| | | $\widetilde{\alpha}^{(pl)}$ | -1.04 | 2.68 | 2.88 | -0.15 | 0.77 | 0.79 | -0.04 | 0.25 | 0.26 |
| | N+N+E | $\widehat{\alpha}^{(ik)}$ | -2.30 | 2.96 | 3.74 | -0.47 | 0.91 | 1.03 | -0.11 | 0.29 | 0.31 |
| | | $\widehat{\alpha}^{(pl)}$ | -10.18 | 4.28 | 11.04 | -4.73 | 2.14 | 5.19 | -1.82 | 0.89 | 2.02 |
| | | $\widehat{\alpha}^{(pl*)}$ | -7.49 | 3.79 | 8.40 | -3.43 | 1.86 | 3.91 | -1.34 | 0.78 | 1.55 |
| | N+N+U | $\widehat{\alpha}^{(ik)}$ | -0.32 | 2.79 | 2.81 | 0.01 | 0.86 | 0.85 | -0.02 | 0.28 | 0.28 |
| | | $\widehat{\alpha}^{(pl)}$ | -3.73 | 2.64 | 4.57 | -1.42 | 0.91 | 1.68 | -0.54 | 0.34 | 0.64 |
| | | $\widehat{\alpha}^{(pl*)}$ | -2.41 | 2.53 | 3.49 | -0.76 | 0.82 | 1.12 | -0.29 | 0.29 | 0.41 |
| | t | $\widehat{\alpha}^{(ik)}$ | -0.46 | 2.90 | 2.94 | 0.02 | 0.86 | 0.86 | -0.02 | 0.28 | 0.28 |
| | | $\widehat{\alpha}^{(pl)}$ | -2.20 | 2.86 | 3.60 | -0.28 | 0.79 | 0.83 | -0.05 | 0.25 | 0.26 |
| | | $\widehat{\alpha}^{(pl*)}$ | -1.93 | 2.82 | 3.41 | -0.23 | 0.79 | 0.82 | -0.04 | 0.25 | 0.26 |

Table 3: Model (2) with Clayton copula, quantities multiplied by 100

| $\tau$ | Marginals | estim | $n = 100$ | | | $n = 1\,000$ | | | $n = 10\,000$ | | |
|---|---|---|---|---|---|---|---|---|---|---|---|
| | | | bias | SD | RMSE | bias | SD | RMSE | bias | SD | RMSE |
| 0.50 | inov | $\widetilde{\alpha}^{(ik)}$ | 0.21 | 3.61 | 3.61 | 0.01 | 1.15 | 1.15 | -0.01 | 0.35 | 0.35 |
| | | $\widetilde{\alpha}^{(pl)}$ | 0.04 | 3.39 | 3.39 | 0.00 | 1.07 | 1.07 | -0.02 | 0.34 | 0.34 |
| | N+N+E | $\widehat{\alpha}^{(ik)}$ | -0.41 | 3.69 | 3.71 | -0.07 | 1.15 | 1.15 | -0.02 | 0.35 | 0.35 |
| | | $\widehat{\alpha}^{(pl)}$ | -0.78 | 3.48 | 3.56 | -0.12 | 1.08 | 1.08 | -0.03 | 0.34 | 0.34 |
| | | $\widehat{\alpha}^{(pl*)}$ | -0.51 | 3.80 | 3.83 | -0.08 | 1.11 | 1.11 | -0.03 | 0.34 | 0.34 |
| | N+N+U | $\widehat{\alpha}^{(ik)}$ | 0.11 | 3.67 | 3.67 | -0.00 | 1.15 | 1.15 | -0.01 | 0.35 | 0.35 |
| | | $\widehat{\alpha}^{(pl)}$ | -0.14 | 3.46 | 3.46 | -0.02 | 1.08 | 1.08 | -0.02 | 0.34 | 0.34 |
| | | $\widehat{\alpha}^{(pl*)}$ | 0.09 | 3.76 | 3.76 | 0.01 | 1.11 | 1.11 | -0.02 | 0.34 | 0.34 |
| | t | $\widehat{\alpha}^{(ik)}$ | -0.20 | 3.69 | 3.69 | -0.04 | 1.15 | 1.15 | -0.02 | 0.35 | 0.35 |
| | | $\widehat{\alpha}^{(pl)}$ | -0.48 | 3.48 | 3.51 | -0.06 | 1.08 | 1.08 | -0.02 | 0.34 | 0.34 |
| | | $\widehat{\alpha}^{(pl*)}$ | -0.17 | 3.79 | 3.79 | -0.02 | 1.11 | 1.11 | -0.02 | 0.34 | 0.34 |
| 0.75 | inov | $\widetilde{\alpha}^{(ik)}$ | 0.06 | 1.91 | 1.91 | -0.01 | 0.56 | 0.56 | -0.00 | 0.17 | 0.17 |
| | | $\widetilde{\alpha}^{(pl)}$ | -0.56 | 1.83 | 1.91 | -0.08 | 0.53 | 0.54 | -0.01 | 0.16 | 0.16 |
| | N+N+E | $\widehat{\alpha}^{(ik)}$ | -1.27 | 2.12 | 2.47 | -0.20 | 0.59 | 0.62 | -0.02 | 0.17 | 0.18 |
| | | $\widehat{\alpha}^{(pl)}$ | -2.18 | 2.15 | 3.06 | -0.32 | 0.57 | 0.65 | -0.04 | 0.16 | 0.17 |
| | | $\widehat{\alpha}^{(pl*)}$ | -2.02 | 2.26 | 3.03 | -0.30 | 0.58 | 0.65 | -0.03 | 0.17 | 0.17 |
| | N+N+U | $\widehat{\alpha}^{(ik)}$ | -0.19 | 1.96 | 1.97 | -0.03 | 0.57 | 0.57 | -0.01 | 0.17 | 0.17 |
| | | $\widehat{\alpha}^{(pl)}$ | -0.90 | 1.88 | 2.08 | -0.11 | 0.53 | 0.54 | -0.01 | 0.16 | 0.16 |
| | | $\widehat{\alpha}^{(pl*)}$ | -0.79 | 1.99 | 2.14 | -0.09 | 0.55 | 0.55 | -0.01 | 0.17 | 0.17 |
| | t | $\widehat{\alpha}^{(ik)}$ | -0.68 | 2.02 | 2.13 | -0.09 | 0.57 | 0.58 | -0.01 | 0.17 | 0.17 |
| | | $\widehat{\alpha}^{(pl)}$ | -1.44 | 1.98 | 2.45 | -0.17 | 0.54 | 0.56 | -0.02 | 0.16 | 0.17 |
| | | $\widehat{\alpha}^{(pl*)}$ | -1.27 | 2.09 | 2.45 | -0.15 | 0.55 | 0.57 | -0.02 | 0.17 | 0.17 |

Table 4: Model (2) with Frank copula, quantities multiplied by 100

| $\tau$ | Marginals | estim | $n = 100$ | | | $n = 1\,000$ | | | $n = 10\,000$ | | |
|---|---|---|---|---|---|---|---|---|---|---|---|
| | | | bias | SD | RMSE | bias | SD | RMSE | bias | SD | RMSE |
| 0.50 | inov | $\widetilde{\alpha}^{(ik)}$ | 0.20 | 4.40 | 4.40 | 0.01 | 1.35 | 1.35 | -0.01 | 0.44 | 0.44 |
| | | $\widetilde{\alpha}^{(pl)}$ | 0.71 | 4.14 | 4.20 | 0.10 | 1.29 | 1.29 | -0.00 | 0.42 | 0.42 |
| | N+N+E | $\widehat{\alpha}^{(ik)}$ | -0.87 | 4.36 | 4.45 | -0.21 | 1.34 | 1.35 | -0.04 | 0.44 | 0.44 |
| | | $\widehat{\alpha}^{(pl)}$ | -2.05 | 3.97 | 4.47 | -1.11 | 1.33 | 1.73 | -0.43 | 0.47 | 0.64 |
| | | $\widehat{\alpha}^{(pl*)}$ | -0.41 | 4.14 | 4.16 | -0.44 | 1.30 | 1.38 | -0.19 | 0.45 | 0.49 |
| | N+N+U | $\widehat{\alpha}^{(ik)}$ | 0.02 | 4.40 | 4.40 | -0.01 | 1.35 | 1.35 | -0.01 | 0.44 | 0.44 |
| | | $\widehat{\alpha}^{(pl)}$ | -0.03 | 4.03 | 4.03 | -0.24 | 1.26 | 1.29 | -0.12 | 0.42 | 0.44 |
| | | $\widehat{\alpha}^{(pl*)}$ | 0.86 | 4.24 | 4.32 | 0.14 | 1.30 | 1.31 | 0.01 | 0.42 | 0.42 |
| | t | $\widehat{\alpha}^{(ik)}$ | 0.16 | 4.42 | 4.42 | 0.01 | 1.35 | 1.35 | -0.01 | 0.44 | 0.44 |
| | | $\widehat{\alpha}^{(pl)}$ | 0.50 | 4.18 | 4.21 | 0.08 | 1.29 | 1.29 | -0.00 | 0.42 | 0.42 |
| | | $\widehat{\alpha}^{(pl*)}$ | 1.01 | 4.30 | 4.41 | 0.22 | 1.31 | 1.32 | 0.04 | 0.42 | 0.43 |
| 0.75 | inov | $\widetilde{\alpha}^{(ik)}$ | 0.18 | 2.66 | 2.66 | -0.02 | 0.82 | 0.82 | -0.00 | 0.25 | 0.25 |
| | | $\widetilde{\alpha}^{(pl)}$ | -0.24 | 2.40 | 2.41 | -0.07 | 0.75 | 0.76 | -0.01 | 0.23 | 0.23 |
| | N+N+E | $\widehat{\alpha}^{(ik)}$ | -1.48 | 2.65 | 3.04 | -0.39 | 0.84 | 0.93 | -0.07 | 0.25 | 0.26 |
| | | $\widehat{\alpha}^{(pl)}$ | -4.76 | 2.80 | 5.52 | -2.23 | 1.21 | 2.54 | -0.85 | 0.48 | 0.97 |
| | | $\widehat{\alpha}^{(pl*)}$ | -3.11 | 2.66 | 4.09 | -1.44 | 1.07 | 1.79 | -0.55 | 0.41 | 0.69 |
| | N+N+U | $\widehat{\alpha}^{(ik)}$ | -0.12 | 2.66 | 2.66 | -0.07 | 0.82 | 0.82 | -0.01 | 0.25 | 0.25 |
| | | $\widehat{\alpha}^{(pl)}$ | -1.44 | 2.34 | 2.75 | -0.67 | 0.79 | 1.04 | -0.26 | 0.27 | 0.37 |
| | | $\widehat{\alpha}^{(pl*)}$ | -0.68 | 2.42 | 2.51 | -0.26 | 0.76 | 0.81 | -0.09 | 0.25 | 0.26 |
| | t | $\widehat{\alpha}^{(ik)}$ | 0.09 | 2.70 | 2.70 | -0.03 | 0.82 | 0.82 | -0.01 | 0.25 | 0.25 |
| | | $\widehat{\alpha}^{(pl)}$ | -0.44 | 2.47 | 2.51 | -0.09 | 0.76 | 0.76 | -0.01 | 0.23 | 0.23 |
| | | $\widehat{\alpha}^{(pl*)}$ | -0.27 | 2.48 | 2.49 | -0.03 | 0.76 | 0.76 | 0.01 | 0.24 | 0.24 |

Table 5: Model (2) with Gumbel copula, quantities multiplied by 100

| $\tau$ | Marginals | estim | $n = 100$ | | | $n = 1\,000$ | | | $n = 10\,000$ | | |
|---|---|---|---|---|---|---|---|---|---|---|---|
| | | | bias | SD | RMSE | bias | SD | RMSE | bias | SD | RMSE |
| 0.50 | inov | $\widetilde{\alpha}^{(ik)}$ | -0.12 | 4.04 | 4.04 | 0.02 | 1.28 | 1.28 | 0.01 | 0.38 | 0.38 |
| | | $\widetilde{\alpha}^{(pl)}$ | 1.02 | 3.66 | 3.80 | 0.19 | 1.19 | 1.20 | 0.03 | 0.36 | 0.36 |
| | N+N+E | $\widehat{\alpha}^{(ik)}$ | -0.74 | 3.96 | 4.03 | -0.10 | 1.28 | 1.29 | -0.01 | 0.38 | 0.38 |
| | | $\widehat{\alpha}^{(pl)}$ | 0.10 | 3.52 | 3.52 | -0.14 | 1.19 | 1.20 | -0.07 | 0.36 | 0.36 |
| | | $\widehat{\alpha}^{(pl*)}$ | 0.91 | 3.83 | 3.93 | 0.14 | 1.22 | 1.23 | 0.03 | 0.36 | 0.36 |
| | N+N+U | $\widehat{\alpha}^{(ik)}$ | -0.26 | 4.04 | 4.05 | -0.00 | 1.28 | 1.28 | 0.01 | 0.38 | 0.38 |
| | | $\widehat{\alpha}^{(pl)}$ | 0.74 | 3.63 | 3.70 | 0.08 | 1.19 | 1.19 | -0.01 | 0.36 | 0.36 |
| | | $\widehat{\alpha}^{(pl*)}$ | 1.34 | 3.87 | 4.10 | 0.31 | 1.22 | 1.25 | 0.08 | 0.36 | 0.37 |
| | t | $\widehat{\alpha}^{(ik)}$ | -0.16 | 4.07 | 4.07 | 0.01 | 1.28 | 1.28 | 0.01 | 0.38 | 0.38 |
| | | $\widehat{\alpha}^{(pl)}$ | 0.95 | 3.67 | 3.79 | 0.18 | 1.19 | 1.20 | 0.03 | 0.36 | 0.36 |
| | | $\widehat{\alpha}^{(pl*)}$ | 1.41 | 3.92 | 4.16 | 0.30 | 1.22 | 1.26 | 0.07 | 0.36 | 0.37 |
| 0.75 | inov | $\widetilde{\alpha}^{(ik)}$ | -0.11 | 2.37 | 2.37 | -0.03 | 0.74 | 0.74 | 0.00 | 0.22 | 0.22 |
| | | $\widetilde{\alpha}^{(pl)}$ | -0.17 | 2.18 | 2.18 | -0.03 | 0.66 | 0.66 | 0.00 | 0.20 | 0.20 |
| | N+N+E | $\widehat{\alpha}^{(ik)}$ | -1.39 | 2.36 | 2.74 | -0.28 | 0.76 | 0.81 | -0.04 | 0.22 | 0.22 |
| | | $\widehat{\alpha}^{(pl)}$ | -2.15 | 2.22 | 3.09 | -0.77 | 0.78 | 1.10 | -0.23 | 0.23 | 0.32 |
| | | $\widehat{\alpha}^{(pl*)}$ | -1.41 | 2.24 | 2.65 | -0.46 | 0.75 | 0.88 | -0.12 | 0.22 | 0.25 |
| | N+N+U | $\widehat{\alpha}^{(ik)}$ | -0.36 | 2.34 | 2.37 | -0.07 | 0.74 | 0.74 | -0.01 | 0.22 | 0.22 |
| | | $\widehat{\alpha}^{(pl)}$ | -0.74 | 2.12 | 2.24 | -0.29 | 0.66 | 0.72 | -0.09 | 0.20 | 0.22 |
| | | $\widehat{\alpha}^{(pl*)}$ | -0.31 | 2.20 | 2.22 | -0.08 | 0.67 | 0.68 | -0.01 | 0.20 | 0.20 |
| | t | $\widehat{\alpha}^{(ik)}$ | -0.14 | 2.36 | 2.36 | -0.03 | 0.74 | 0.74 | 0.00 | 0.22 | 0.22 |
| | | $\widehat{\alpha}^{(pl)}$ | -0.23 | 2.18 | 2.19 | -0.03 | 0.66 | 0.66 | 0.00 | 0.20 | 0.20 |
| | | $\widehat{\alpha}^{(pl*)}$ | -0.09 | 2.23 | 2.23 | 0.01 | 0.68 | 0.68 | 0.02 | 0.20 | 0.20 |

Table 6: Model (2) with Gaussian copula, quantities multiplied by 100

| $\tau$ | Marginals | estim | $n=100$ | | | $n=1\,000$ | | | $n=10\,000$ | | |
|---|---|---|---|---|---|---|---|---|---|---|---|
| | | | bias | SD | RMSE | bias | SD | RMSE | bias | SD | RMSE |
| 0.50 | inov | $\widetilde{\alpha}^{(ik)}$ | 0.06 | 4.42 | 4.41 | 0.01 | 1.39 | 1.38 | -0.00 | 0.44 | 0.44 |
| | | $\widetilde{\alpha}^{(pl)}$ | 0.97 | 4.20 | 4.31 | 0.15 | 1.34 | 1.35 | 0.02 | 0.42 | 0.42 |
| | N+N+E | $\widehat{\alpha}^{(ik)}$ | -0.69 | 4.36 | 4.41 | -0.13 | 1.38 | 1.39 | -0.02 | 0.44 | 0.44 |
| | | $\widehat{\alpha}^{(pl)}$ | -0.42 | 4.10 | 4.12 | -0.37 | 1.34 | 1.39 | -0.14 | 0.42 | 0.45 |
| | | $\widehat{\alpha}^{(pl*)}$ | 0.46 | 4.29 | 4.32 | 0.02 | 1.36 | 1.36 | -0.00 | 0.42 | 0.42 |
| | N+N+U | $\widehat{\alpha}^{(ik)}$ | -0.17 | 4.43 | 4.44 | -0.02 | 1.39 | 1.39 | -0.01 | 0.44 | 0.44 |
| | | $\widehat{\alpha}^{(pl)}$ | 0.35 | 4.15 | 4.17 | -0.08 | 1.33 | 1.33 | -0.06 | 0.42 | 0.42 |
| | | $\widehat{\alpha}^{(pl*)}$ | 1.03 | 4.34 | 4.45 | 0.26 | 1.35 | 1.38 | 0.06 | 0.42 | 0.42 |
| | t | $\widehat{\alpha}^{(ik)}$ | -0.02 | 4.45 | 4.45 | 0.01 | 1.39 | 1.39 | -0.00 | 0.44 | 0.44 |
| | | $\widehat{\alpha}^{(pl)}$ | 0.83 | 4.24 | 4.32 | 0.13 | 1.35 | 1.35 | 0.02 | 0.42 | 0.42 |
| | | $\widehat{\alpha}^{(pl*)}$ | 1.24 | 4.32 | 4.50 | 0.32 | 1.35 | 1.39 | 0.08 | 0.42 | 0.43 |
| 0.75 | inov | $\widetilde{\alpha}^{(ik)}$ | -0.29 | 2.71 | 2.72 | 0.03 | 0.82 | 0.82 | 0.00 | 0.26 | 0.26 |
| | | $\widetilde{\alpha}^{(pl)}$ | -0.31 | 2.44 | 2.46 | 0.01 | 0.77 | 0.77 | -0.00 | 0.24 | 0.24 |
| | N+N+E | $\widehat{\alpha}^{(ik)}$ | -1.64 | 2.69 | 3.15 | -0.26 | 0.83 | 0.87 | -0.05 | 0.26 | 0.27 |
| | | $\widehat{\alpha}^{(pl)}$ | -2.53 | 2.50 | 3.55 | -0.90 | 0.86 | 1.24 | -0.31 | 0.29 | 0.42 |
| | | $\widehat{\alpha}^{(pl*)}$ | -1.85 | 2.53 | 3.13 | -0.58 | 0.83 | 1.01 | -0.20 | 0.28 | 0.34 |
| | N+N+U | $\widehat{\alpha}^{(ik)}$ | -0.58 | 2.68 | 2.74 | -0.02 | 0.81 | 0.81 | -0.01 | 0.26 | 0.26 |
| | | $\widehat{\alpha}^{(pl)}$ | -1.16 | 2.37 | 2.64 | -0.41 | 0.77 | 0.87 | -0.16 | 0.25 | 0.30 |
| | | $\widehat{\alpha}^{(pl*)}$ | -0.66 | 2.45 | 2.53 | -0.11 | 0.76 | 0.77 | -0.05 | 0.24 | 0.25 |
| | t | $\widehat{\alpha}^{(ik)}$ | -0.27 | 2.72 | 2.73 | 0.04 | 0.81 | 0.82 | 0.00 | 0.26 | 0.26 |
| | | $\widehat{\alpha}^{(pl)}$ | -0.34 | 2.48 | 2.50 | 0.01 | 0.77 | 0.77 | -0.00 | 0.24 | 0.24 |
| | | $\widehat{\alpha}^{(pl*)}$ | -0.25 | 2.49 | 2.50 | 0.07 | 0.77 | 0.77 | 0.02 | 0.24 | 0.24 |

Table 7: Model (2) with Student copula, quantities multiplied by 100
